# Supplementary material for: Many-particle Entanglement in Multiple Quantum NMR Spectroscopy
Source: arXiv:2001.10607 source file (2020-01-28)
Supplement: Supplementary file 1 [file appendix.tex]

\appendix
\section{Appendix}
Taking into account that $n^2 \leq N^2$ and $sum_n J_{\mathrm{lT}, n}(\tau)=1$ one can obtain a simple estimation. 
\begin{equation} 
    M_2(\tau) \leq N^2.
\end{equation}
The more subtle estimation requires using the properties of the density matrix.
\par 
We rewrite Eq.~(\ref{eq:dispersion}) as 
\begin{equation}
    M_2(\tau) = \sum\limits_{i < j}
    (i - j)^2 \left|\rho^{ij}_{\mathrm{LT}}\right|^2.
\end{equation}
Since $\rho_{\mathrm{LT}}$ is a positive semi-definite operator, we have 
\begin{equation}
    \rho_{\mathrm{LT}}^{ii}\rho_\mathrm{LT}^{jj} -
    \left|\rho^{ij}_{\mathrm{LT}}\right|^2 \beq 0.
\end{equation}
Then 
\begin{multline}
    M_2(\tau) \leq 
    \sum\limits_{i < j}
    \rho_{\mathrm{LT}}^{ii}\rho_{\mathrm{LT}}^{jj}
    (j - i)^2  \leq 
    N^2 \sum\limits_{i < j}
    \rho_{\mathrm{LT}}^{ii}\rho_{\mathrm{LT}}^{jj} = 
    \frac 1 2 N^2 \sum\limits_{i,j}
    \rho_{\mathrm{LT}}^{ii}\rho_{\mathrm{LT}}^{jj} = 
    \frac 1 2 N^2 
    \sum\limits_{i} \rho_{\mathrm{LT}}^{ii}
    \sum\limits_{j} \rho_{\mathrm{LT}}^{jj}
\end{multline}

Since the density matrix is an operator of trace one, 
\begin{equation}
	\sum\limits_{i} \rho_{\mathrm{LT}}^{ii} = 
	\sum\limits_{j} \rho_{\mathrm{LT}}^{jj} = 
	1
\end{equation}
and we obtain
\begin{equation}
	M_2(\tau) \leq \dfrac{N^2}{2}
\end{equation}
This inequality result in $F_\mathrm{Q} \leq N^2$ as in \cite{fisher_and_entanglement}.
